# Supplementary material for: Compression and In-Situ Query Processing for Fine-Grained Array Lineage
Source: arXiv:2405.17701 source file (2024-05-27)
Supplement: Supplementary file 1 [file appendix.tex]

\section{Experimental Implementation}
In principle, \sys is agnostic to the provenance capture methodology. We provide an API for storage, indexing, and query processing. In the implementation,  we integrate \sys with the \texttt{Python} data science stack and track provenance in \texttt{numpy} arrays and \texttt{pandas} data frames. Here, we will describe the main mechanism we use to capture provenance using a technique we call annotated execution.

The basic idea of annotation-based capture is to embed tracking information in every element so that the tracking information is propagated through to the final result when the element is manipulated. 
We assume that every user-defined function takes as input a set of multidimensional \texttt{cell} arrays and returns a set of multidimensional \texttt{cell} arrays(or cast appropriately to make this so).
\texttt{cell} is some pre-defined super data type that covers all interesting scenarios.

Suppose we extended the \texttt{cell} type to be an \texttt{annotated\_cell}, which is a struct of a \texttt{cell} data value and a set of annotations. 
Now, let \texttt{op} be an n-array operation over \texttt{cell} values --- it takes n \texttt{cell} values as input and outputs a single \texttt{cell}. The \texttt{annotated\_cell} data type has the following semantics for \texttt{op}: 
\begin{lstlisting}
def apply(op, others):
    v = [o.data for o in others]
    a = [o.annotations for o in others]
    return annotated_double(op(v), union(a))
\end{lstlisting}
It applies the function to all data values and takes a union of all their annotations. This basic structure can override the primitive numerical operations used to manipulate \texttt{cell} data types such as addition, subtraction, multiplication, division, etc.
With the custom data type API in \texttt{numpy}~\footnote{https://numpy.org/doc/stable/reference/arrays.dtypes.html, https://numpy.org/doc/stable/user/basics.ufuncs.html}, there are a relatively small number of operations that have to be overridden to make such an annotated double compatible with a vast majority of the library.

We use these data types to track function provenance over arrays as follows. Given a function and set of input arrays, each array is converted into a \texttt{annotated\_cell} array. Each element is initialized to have its original value as its data value, and the annotation is the singleton set of its current position in the input array. We have to further tag these positions with a unique identifier of which input array.
The provenance accumulates in the elements annotations as \texttt{numpy} operations are applied to the annotated arrays.
Therefore, at the output, each element contains a complete history of the other elements that contributed to it. 

This structure is particularly well-suited for array programming environments because almost all of the core operations are numerical, where if the input is a \texttt{cell} array, the output is also a \texttt{cell} array or could be cast into one (e.g., a Boolean array).  
Of course, it is always possible to obfuscate the provenance with operations that change the data type or leverage structures unknown to \texttt{numpy} - e.g., by serializing the entire array into a string, manipulating on that string, and then deserializing.
In our first implementation, we ignore such problems. 
We treat the capturing system as a best-effort provenance graph that assumes users stay within numerical and \texttt{numpy} array operations.

\subsubsection{In-Memory Annotation Format}
Our implementation is written in C - for efficient computation and low-level memory management - and linked through Python's C interface. Each annotation tuple is represented with three 32-bit integers. Its first value is the array id, and its second and third values are array indices. This defines a unique cell for an array of up to 2-d dimensions (though the basic strategy extends to any dimensionality). These tuples are laid out into a C array and copied during operations. The first value of the array is directly stored in the \texttt{annotated\_cell} data type, and the rest is stored as a pointer to a dynamically allocated memory buffer. For specific functions, our system supports pre-allocating a consistent memory buffer to avoid frequent memory requests.

\section{Implementation Benchmarks}
We believe that our provenance capture framework offers state-of-the-art performance for the Python data science stack. Here we illustrate the costs (additional cost over normal execution) of capturing this provenance. 
These numbers are informative because they put the storage optimizations into absolute context.

\subsection{Experiment Design} \label{sec:workload}

\begin{table*}[ht]
\footnotesize
    \centering
    \begin{tabularx}{1.9\columnwidth}{l|lllll}
    \hline
      &Operation Name   &  \texttt{numpy} & Input Arrays Size & Output Arrays Size & Notes \\
     \hline
      1 & Negative  &  negative & X: (10, 100000) & Z: (10, 100000) & element-wise \\
      2 & Addition  &  add & X: (10, 100000), Y:(10, 100000) & Z: (10, 100000) & element-wise over two inputs \\
      3 & Aggregate  &  sum & X: (1000, 1000), & Z: (1000, 1) & one axis aggregation \\
   4 & Repetition  &  tile(reps=(2,2)) & X: (10, 100000) & Z: (20, 200000) & duplicate array 4 times \\
    5 & MatMul  &  dot & X: (1000, 1000), Y: (1000, 1000) & Z: (1000,1000) & linear algebra matrix product \\
    6 & MatVecMul  &  dot & X: (1000, 1000), Y: (1000, ) & Z: (1000) & linear algebra matrix-vector product \\
    7 & VecMul  &  dot & X: (1000, ), Y: (1000, ) & Z: (1, ) & linear algebra vector dot product \\
    \hline
   8 & RandFilter  &  - & X: (1000000, 1) & Z: (1000000, 1) & filter elements greater than average on a randomly generated array \\
    9 & CorrFilter  &  - & X: (1000000, 1) & Z: (1000000, 1) & filter elements greater than average on a correlated array \\
    10 & ImgFilter  &  - & X: (1000, 1000) & Z: (1000, 1000) & filter non-zero elements on upscaled MNIST image\\
    11 & RandBin4  &  - & X: (1000000, 1) & Z: (4, ) & divide a randomly generated array into 4 bins \\
    12 & SortBin4  &  - & X: (1000000, 1) & Z: (4, ) & divide a sorted array into 4 bins \\
    \end{tabularx}
    \vspace{5pt}
    \caption{Description of \protect\texttt{numpy}-based Operations Used in Capture Evaluation \label{apx:np_functions}}
\end{table*}

 We simulate the example in the introduction where a user wants to understand the provenance relationships in contributor code in an array programming library for these array operations. We select 12 \texttt{numpy} operations that range from typical in prior work (linear algebra) to less well-studied (histogram construction). \sys does not know how these operations behave beforehand. Seven operations are data-independent (the provenance is independent of the array's values), and five are data-dependent. Table \ref{apx:np_functions} summarizes these operations in detail. For the data-dependent operations, we will briefly describe the content of their array to give an intuition of the operation's provenance relation. $X_{\text{RandFilter}}$ and $X_\text{RandBin4}$ are drawn randomly from $[0, 1]$. For every cell, $c[i]$, in $X_{\text{CorrFilter}}$, we have $c[i] = \mathcal{N}(i, m/10)$, where $m = 100000000$ is the first dimension size. We also draw $X_{\text{SortedBin4}}$ from $[0, 1]$, but then sort the elements physically. $X_{\text{ImgFilter}}$ is an up-scaled MNIST image of a handwritten digit that is 0 for all elements in the background.

The primary metric is overhead over standard \texttt{numpy} execution.
We consider two function types for additional microbenchmark performance tests: a one-to-one element-wise operation and one-axis aggregation functions. These show extremes in how many input cells correlated to output cells - only a single input in the first case and along a whole dimension in the second case.

\subsection{Capture Time}
In our first experiment, we evaluate our annotated execution environment on our workload. Note, we did not modify the \texttt{numpy} functions in any way to capture this information other than registering them to \sys. 
Figure \ref{fig:annotated_exec} shows the results of our workload executed over 1M element input arrays.
We find that the cost of annotated execution is steep in relative terms (sometimes 40x slower than the standard execution). 
However, in absolute terms, the differences are relatively small considering the debugging (less than 100ms for every operation other than o5) and introspection benefits provenance provides.

\subsection{Micro-Benchmark Baselines}
Secondly, we compared the performance of \sys on the annotated execution to two baseline systems. To the best of our knowledge, there does not currently exist another system with this type of annotation for direct comparison, so this set of experiments serves more as an ablation study.
\begin{itemize}
    \item \textbf{Python Baseline. } A Python-implemented baseline that supports the exact behavior of element annotation as our \sys implementation. It tracks all provenance with Python bindings and function overrides in \textsf{numpy}.
    \item \textbf{C Baseline. } A baseline that extends the Python baseline but uses C data types to track the provenance. It supports the exact behavior of \sys but without our optimization of a pre-allocated buffer.
\end{itemize}

\begin{figure}[t]
    \centering
    \includegraphics[width=0.9\columnwidth]{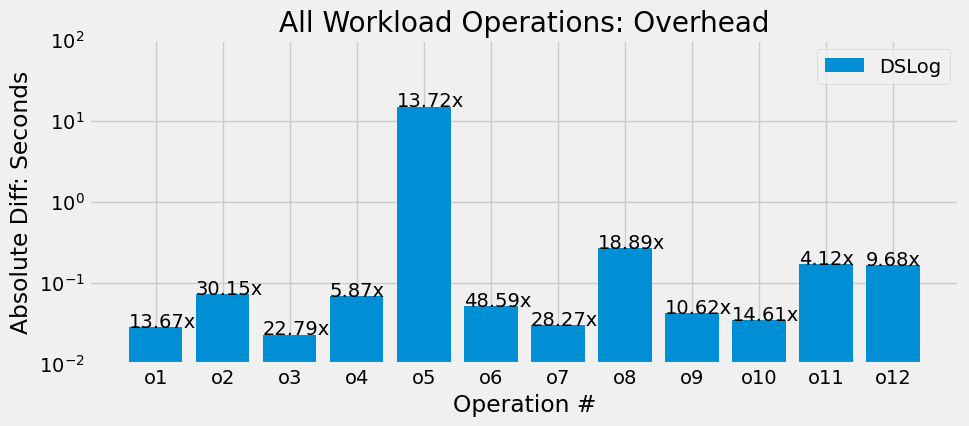}
    \caption{The overhead of annotated execution on 1M cell inputs. Annotated execution adds significant overhead relative to fast operations, but this overhead is still small in absolute terms.}
    \label{fig:annotated_exec}
\end{figure}

\subsection{Deep Diving Performance}

\begin{figure}[t]
  \centering
  \includegraphics[width=.49\columnwidth]{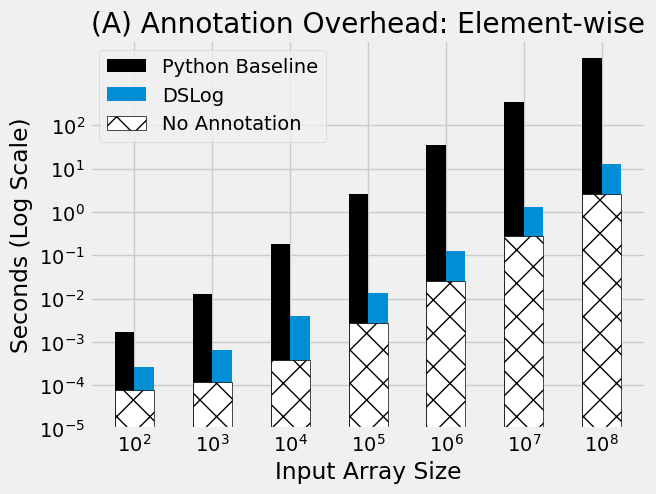}
  \includegraphics[width=.49\columnwidth]{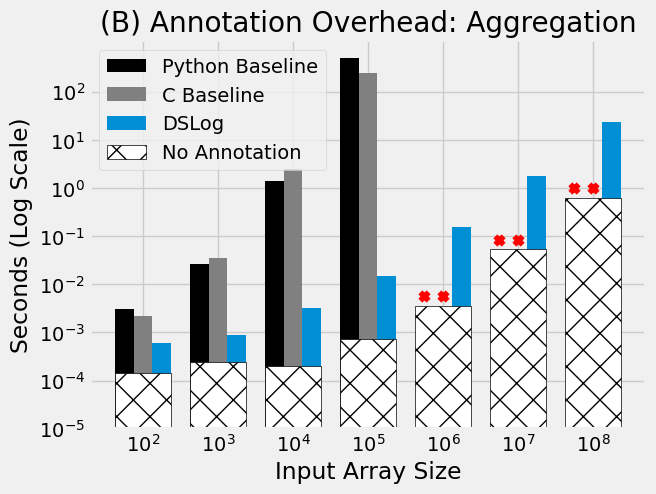}
    \caption{(A) The annotation overhead of element-wise operations, (B) the annotation overhead of aggregation operations.}
    \label{exp:annotate}
\end{figure}

We show that baseline approaches cannot even match the high overheads seen in the last experiment -- they are infeasible at any real scale. 
Figure \ref{exp:annotate} shows the cost of execution for the baselines of an element-wise function and an aggregation function. Figure \ref{exp:annotate}(A) shows the ``easy case'' of this problem, where the amount of annotations for each output element is minimal (only a single input). 
In this case, the C baseline and \sys have equivalent performance; thus, we omit the C baseline. On the element-wise function, \sys performs up 275x faster than the Python baseline, but is still up to 5x slower than the bare function.

Figure \ref{exp:annotate}(B) is more exciting and shows the other extreme of annotated execution, where each output element contains annotations from input cells along a whole axis.
Figure \ref{exp:annotate}(B) shows that, without optimizations, the baselines fail at large scales, we even see this for our C baseline without our optimization of a pre-allocated buffer.
This is because they reallocate new memory for every binary operation within reduce. 

On the aggregate function, \sys performs up to 34000x faster than the Python baseline but is up to 44x slower than running without annotation.
We have demonstrated that detailed low-level memory management can lead to a marked improvement over baseline, but annotation on every cell is inherently costly.
We also note that \sys can scale to large array sizes more efficiently than the baselines. It can maintain a consistent relative overhead on element-wise functions, while relative overhead in the Python implementation increases dramatically. 

\subsection{Function Registration Cost}

\begin{figure}
    \centering
    \includegraphics[width=0.5\columnwidth]{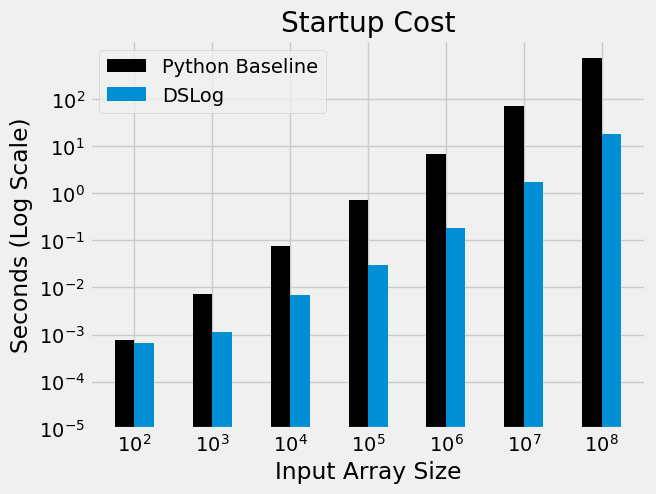}
    \caption{To use annotated execution, input arrays need to be converted to annotated arrays. Without optimization, this can be a significant overhead.}
    \label{exp:init}
\end{figure}
A hidden cost in annotated execution is initialization time, or the time needed to convert the input arrays from their numerical data types into their annotated data types (one can think of this as running an additional element-wise function!). This was included in our workflow experiment but not captured in the micro-benchmarks. Figure \ref{exp:init} shows the cost of annotation initialization for both the Python baseline and \sys's implementation (the annotated initialization cost for the C-baseline would be the same as \sys). This includes the time to convert the array's data type from \texttt{double} to \texttt{annotated\_double} and the time to fill the initial annotation with each cell's current index. We can see from the figure that \sys performs an order of magnitude better than the Python baseline. The Python baseline requires initializing a whole Python object for each cell. In contrast, \sys directly implements a \texttt{numpy} data type stored within the array -- this is interfaced to Python with a C API. Results suggest that the overhead of dealing with the Python object is responsible for most of this performance difference. Both implementations have a performance roughly linear to the number of cells, which is expected since filling the initial annotation requires iteration over all cells.
